# Supplementary material for: Probabilistic Contrastive Learning for Domain Adaptation
Source: arXiv:2111.06021 source file (2024-06-08)
Supplement: Supplementary file 2 [file ssda_officehome_3_shot_appendix.tex]

\begin{table*}[ht]

\centering
\resizebox{\linewidth}{!}{
\begin{tabular}{c|l@{}|cccccccccccc|c}
\specialrule{.1em}{.05em}{.05em}
Net & Method & R$\rightarrow$C & R$\rightarrow$P & R$\rightarrow$A & P$\rightarrow$R & P$\rightarrow$C & P$\rightarrow$A & A$\rightarrow$P & A$\rightarrow$C & A$\rightarrow$R & C$\rightarrow$R & C$\rightarrow$A & C$\rightarrow$P & Mean \\
\hline
\multirow{9}{*}{A} %& S+T & 44.6 & 66.7 & 47.7 & 57.8 & 44.4 & 36.1 & 57.6 & 38.8 & 57.0 & 54.3 & 37.5 & 57.9 & 50.0 \\
% & DANN(JMLR'17) & 47.2 & 66.7 & 46.6 & 58.1 & 44.4 & 36.1 & 57.2 & 39.8 & 56.6 & 54.3 & 38.6 & 57.9 & 50.3 \\
% & ENT(Neurips'05) & 44.9 & 70.4 & 47.1 & 60.3 & 41.2 & 34.6 & 60.7 & 37.8 & 60.5 & 58.0 & 31.8 & 63.4 & 50.9 \\
 %& MME (ICCV'19)~\cite{saito2019semi} & 51.2 & 73.0 & 50.3 & 61.6 & 47.2 & 40.7 & 63.9 & 43.8 & 61.4 & 59.9 & 44.7 & 64.7 & 55.2 \\
 %& Meta-MME (ECCV'20)~\cite{li2020online} & 50.3 & - & - & - & 48.3 & 40.3 & - & 44.5 & - & - & 44.5 & - & - \\
 %& BiAT (IJCAI'20)~\cite{2020Bidirectional} & - & - & - & - & - & - & - & - & - & - & - & - & 56.4 \\
 & APE (ECCV'20)~\cite{Kim2020AttractPA} & 51.9 & 74.6 & 51.2 & 61.6 & 47.9 & 42.1 & 65.5 & 44.5 & 60.9 & 58.1 & 44.3 & 64.8 & 55.6 \\
 & CLDA (NeurIPS'21)~\cite{singh2021clda} & 51.5 & 74.1 & 54.3 & 67.0 & 47.9 & \bf{47.0} & 65.8 & 47.4 & 66.6 & 64.1 & 46.8 & 67.5 & 58.3 \\
  & MME$^{*}$~\cite{saito2019semi} & 44.6 & 73.0 & 50.4 & 62.9 & 48.3 & 41.0 & 63.4 & 45.4 & 62.2 & 60.8 & 43.3 & 65.2 & 55.7 \\ 
 & + \textbf{Our PCL} & 52.8 & 74.7 &  53.7 & 64.6 & 48.9 & 44.5 & 66.3 & 47.1 & 65.0 & 64.8 & 46.4 & 67.9 & 58.1 \\  
\cline{2-15} 
 & CDAC$^\dag$ (CVPR'21)~\cite{li2021cdac} &  54.9 & \textbf{75.8} & 51.8 & 64.3 & 51.3 & 43.6 & 65.1 & 47.5 & 63.1 & 63.0 & 44.9 & 65.6 & 56.8 \\
 & ECACL-P$^\dag$ (ICCV'21)~\cite{li2021ecacl} &  55.4 & 75.7 & \textbf{56.0} & 67.0 & \textbf{52.5} & 46.4 & 67.4 & 48.5 & 66.3 & 60.8 & 45.9 & 67.3 & 59.1 \\
 & MME$^\dag$ & 54.4 & \textbf{75.8} &  54.6 & 66.9 & 52.0 & 45.9 & \textbf{69.2} & \textbf{49.2} & 65.4 & 65.3 & 47.7 & 65.6 & 59.3 \\  
 & + \textbf{Our PCL} & \textbf{55.6} & 75.6 & 55.6 & \textbf{67.8} & 52.0 & 46.4 & 68.8 & 49.0 & \textbf{67.1} & \textbf{67.0} & \textbf{47.9} & \textbf{69.5} & \textbf{60.2} \\ 
\hline
\hline
\multirow{8}{*}{R} %& S+T & 55.7 & 80.8 & 67.8 & 73.1 & 53.8 & 63.5 & 73.1 & 54.0 & 74.2 & 68.3 & 57.6 & 72.3 & 66.2 \\
% & DANN(JMLR'17) & 57.3 & 75.5 & 65.2 & 69.2 & 51.8 & 56.6 & 68.3 & 54.7 & 73.8 & 67.1 & 55.1 & 67.5 & 63.5 \\
% & ENT(Neurips'05) & 62.6 & 85.7 & 70.2 & 79.9 & 60.5 & 63.9 & 79.5 & 61.3 & 79.1 & 76.4 & 64.7 & 79.1 & 71.9 \\
 %& MME (ICCV'19)~\cite{saito2019semi} & 64.6 & 85.5 & 71.3 & 80.1 & 64.6 & 65.5 & 79.0 & 63.6 & 79.7 & 76.6 & 67.2 & 79.3 & 73.1 \\
 %& Meta-MME (ECCV'20)~\cite{li2020online} & 65.2 & - & - & - & 64.5 & 66.7 & - & 63.3 & - & - & 67.5 & - & - \\
 & APE (ECCV'20)~\cite{Kim2020AttractPA} & 66.4 & 86.2 & 73.4 & 82.0 & 65.2 & 66.1 & 81.1 & 63.9 & 80.2 & 76.8 & 66.6 & 79.9 & 74.0 \\
  & CLDA (NeurIPS'21)~\cite{singh2021clda} & 66.0 & 87.6 & 76.7 & 82.2 & 63.9 & 72.4 & 81.4 & 63.4 & 81.3 & 80.3 & 70.5 & 80.9 & 75.5 \\
  & MME$^{*}$~\cite{saito2019semi} & 66.0 & 86.0 & 72.3 & 80.4 & 64.0 & 67.4 & 79.8 & 64.0 & 77.9 & 77.1 & 66.6 & 80.0 & 73.5 \\
  & + \textbf{Our PCL} & 65.4 & 86.7 & 74.5 & 83.1 & 62.9 & 71.0 & 82.8 & 63.7 & 81.0 & 81.1 & 71.0 & 83.1 & 75.5 \\
  \cline{2-15}
 & CDAC$^\dag$ (CVPR'21)~\cite{li2021cdac} & 67.8 & 85.6 & 72.2 & 81.9 & 67.0 & 67.5 & 80.3 & 65.9 & 80.6 & 80.2 & 67.4 & 81.4 & 74.8 \\  
   & MCL$^\dag$ ( IJCAI'22 )~\cite{yan2022multi} & \textbf{70.1} & 88.1 & 75.3 & 83.0 & \textbf{68.0} & 69.9 & 83.9 & 67.5 & \textbf{82.4} & 81.6 & 71.4 & \textbf{84.3} & 77.1 \\ 
  & MME$^\dag$ & 67.2 & 88.1 &  76.6 & 83.0 & 66.8 & 73.6 & 83.8 & 67.3 & 80.5 & 81.1 & 71.8 & 82.7 & 76.9 \\  
 & + \textbf{Our PCL}  & 69.1 & \textbf{89.5} & \textbf{76.9} & \textbf{83.8} & \textbf{68.0} & \textbf{74.7} & \textbf{85.5} & \textbf{67.6} & 82.3 & \textbf{82.7} & \textbf{73.4} & 83.4 & \textbf{78.1} \\ 
\specialrule{.1em}{.05em}{.05em}
\end{tabular}}

\vspace{-2.0mm}
\caption{Accuracy(\%) on \textit{Office-Home} under the setting of 3-shot using Alexnet (A) and Resnet34 (R) as backbone networks. ${\dag}$ means using Fixmath and ${*}$ means our reimplementation.}
\label{tab:ssda_officehome_3_shot_app}
\end{table*}
